# Supplementary material for: OnlineSI: Taming Large Language Model for Online 3D Understanding and Grounding
Source: arXiv:2601.16538 source file (2026-03-06)
Supplement: Supplementary file 1 [file 7_supplementary.tex]

\clearpage
\setcounter{page}{1}
\maketitlesupplementary

\section{More Implementation Details}

\subsection{Spatial Memory Management}

In Sec.~\ref{sec:memory_management}, to maintain a fixed size for $\textbf{M}_t$ and prevent rapid forgetting, we automatically adjust the fusion ratio based on timestep $t$. Here we formulate the fusion process. Following the notations in Sec.~\ref{sec:memory_management}, we reformulate Eq.~\ref{eq:memory_management} as:
\begin{align}
    &\textbf{P}_t = \text{Sample}(\text{Concat}(\textbf{P}_{t-1}, \text{Sample}(\textbf{X}'_t, \alpha_t)), \beta_t),\ \textbf{P}_0 = \emptyset, \\
    &\textbf{S}_t = \text{Sample}(\text{Concat}(\textbf{S}_{t-1}, \text{Sample}(\textbf{Y}_t, \alpha_t)), \beta_t),\ \textbf{S}_0 = \emptyset,
\end{align}
Here $\text{Sample}(\textbf{A}, \alpha)$ means sampling \textbf{A} at ratio $\alpha$, $\text{Concat}(\cdot, \cdot)$ means concatenating two inputs. Assume we set the maximum memory limit to accommodate $N$ frames of input, then we have:
\begin{align}
    &\alpha_t = \begin{cases}
        1, \quad t\leq N \\
        \frac{N}{t - 1}, \quad t > N
    \end{cases} \\
    &\beta_t = \begin{cases}
        1, \quad t\leq N \\
        \frac{t-1}{t}, \quad t > N
    \end{cases}
\end{align}
It's easy to verify that this ensures a fixed upper limit for memory size, and that each input frame occupies the same proportion in memory.

\subsection{Point Cloud Encoder and Semantic Encoder}

\begin{figure*}[htbp]
    \centering
    \includegraphics[width=\linewidth]{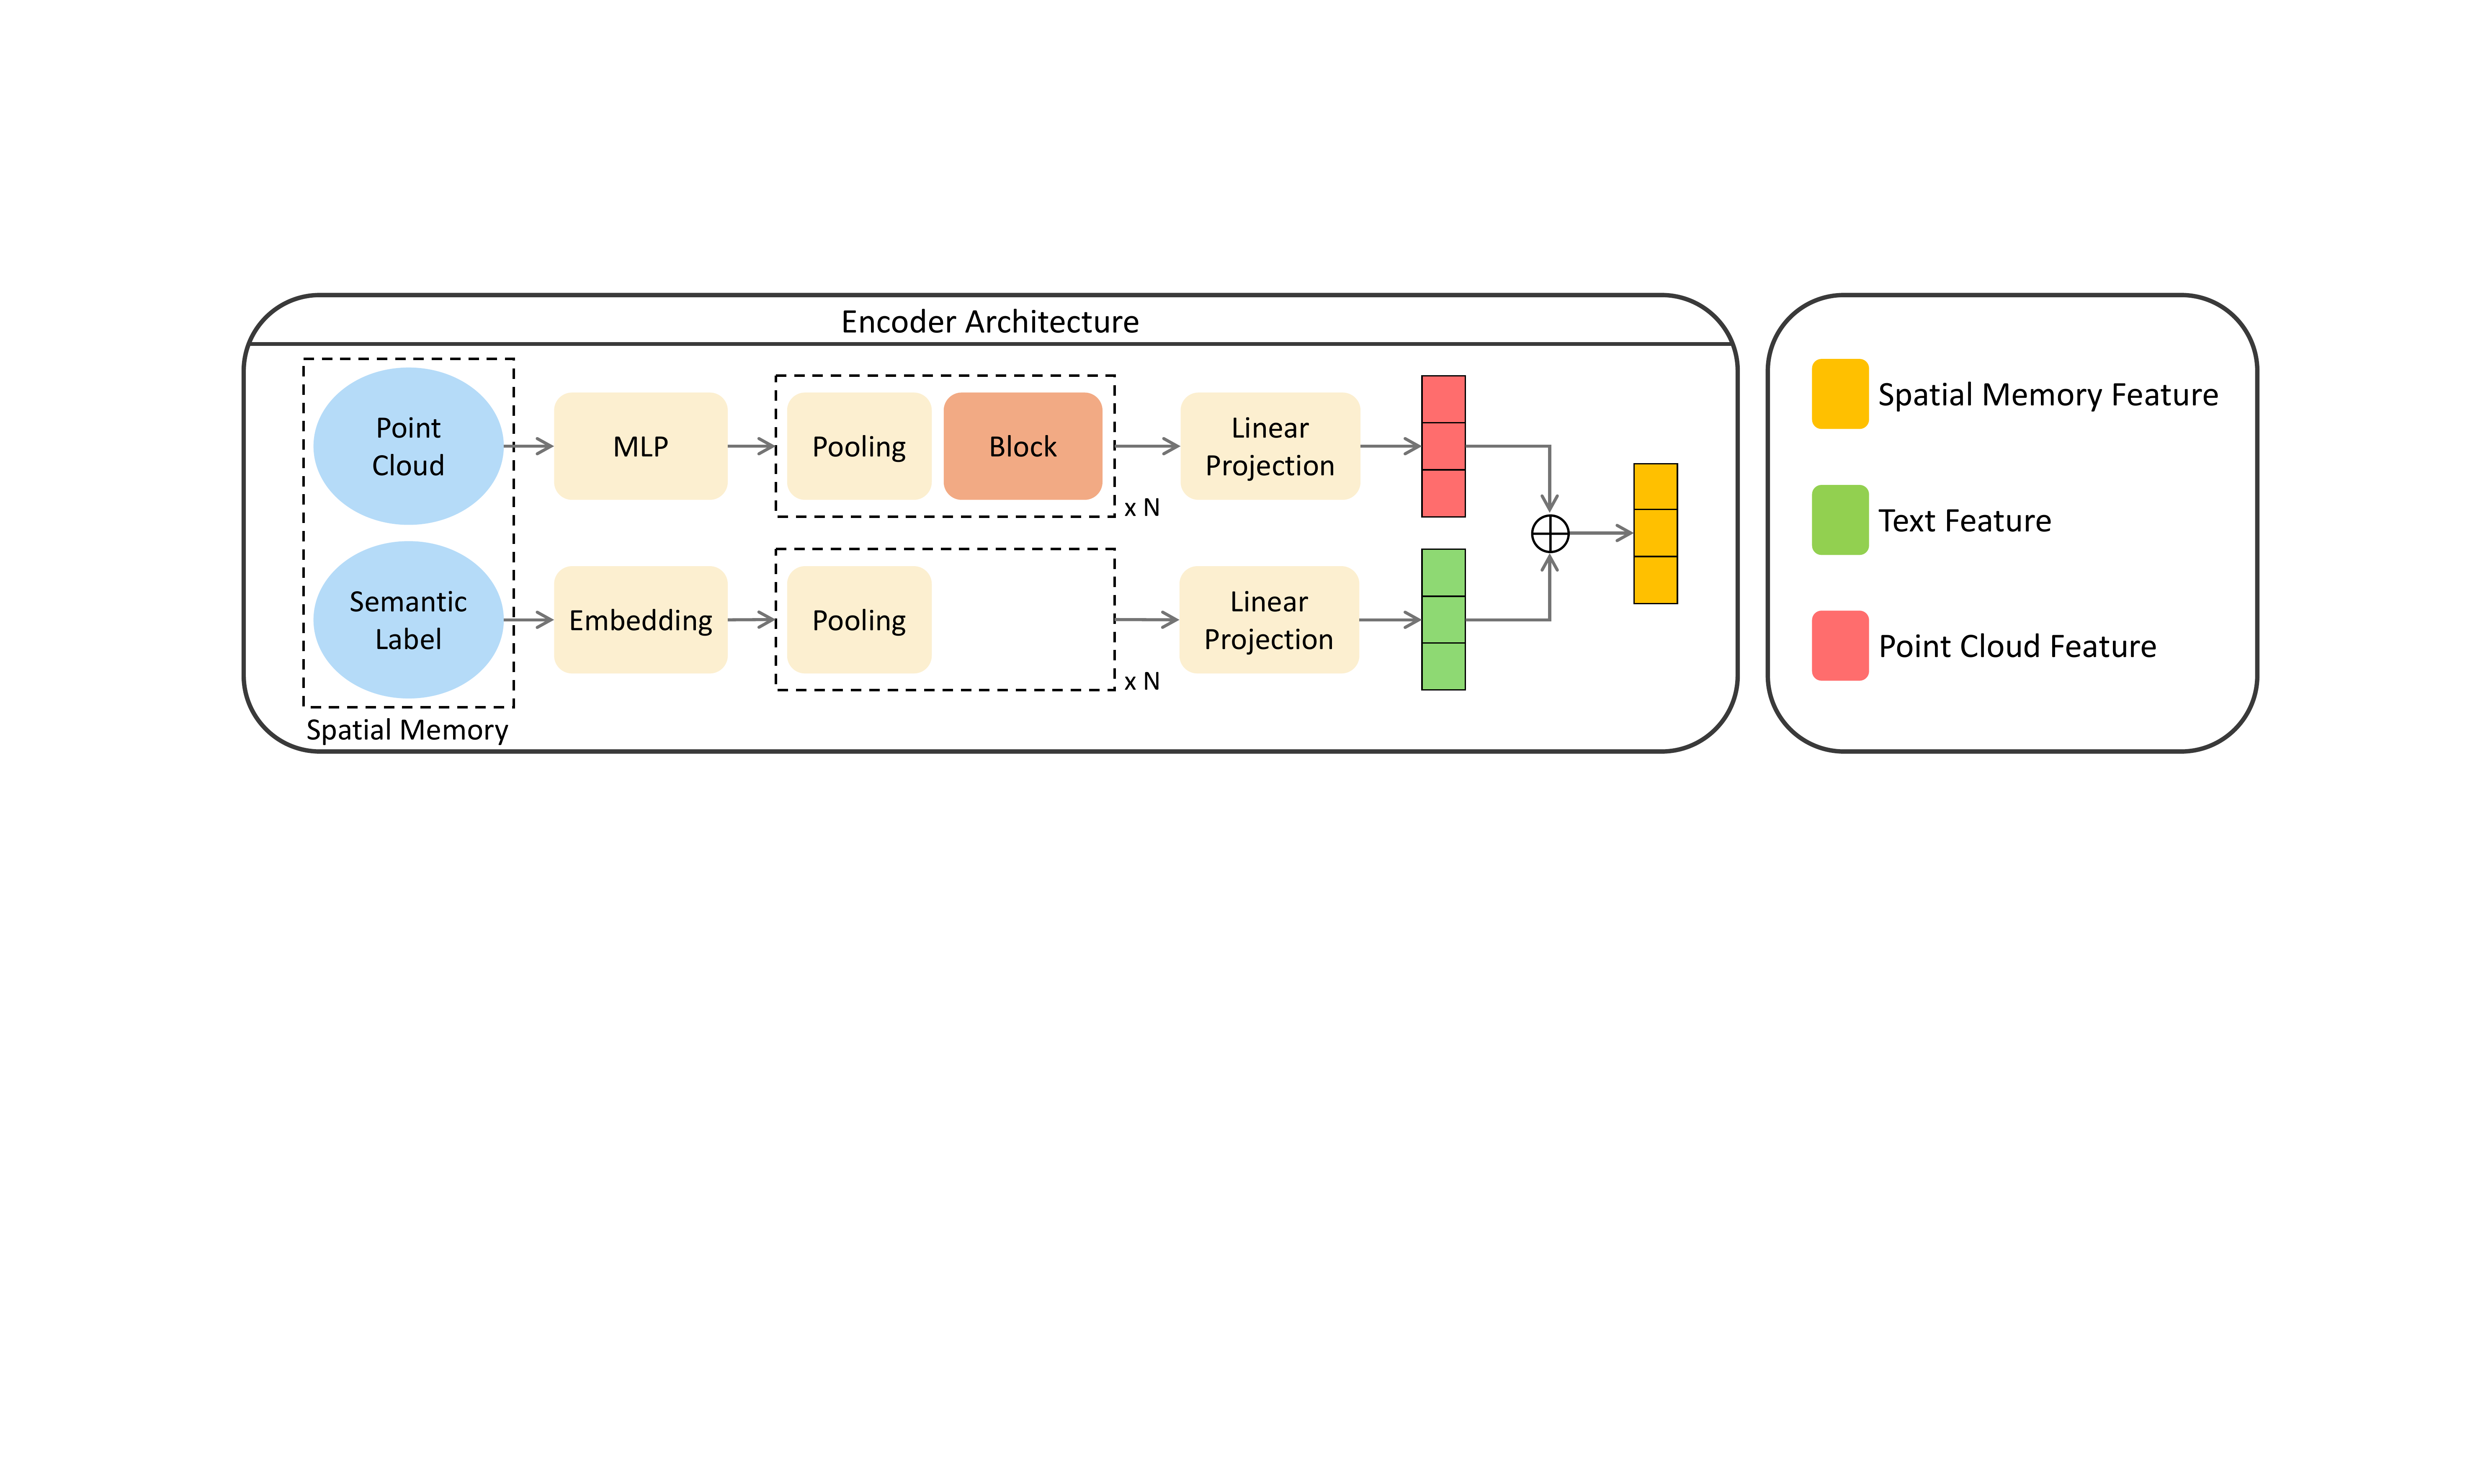}
    \caption{\textbf{Point Cloud Encoder and Semantic Encoder.} For the semantic encoder, we first transform the semantic label into text features through embedding operations, and then obtain semantic feature patches through pooling operations with the same structure as Sonata.}
    \label{fig:encoders}
\end{figure*}

Here we further elaborate on the design of the semantic encoder. As shown in Fig.~\ref{fig:encoders}, the point cloud encoder follows the design in Sonate~\cite{wu2025sonata}. For the semantic encoder, in the embedding layer we first leverage Llama's tokenizer to divide the semantic label into tokens of variable length, and then take the average of these token features as the corresponding text feature. We then use only the pooling operations to aggregate these per-point features into semantic feature patches, and fine-tune only the last linear projection layer for the fusion of different representations.

\section{More Experiment Details}

\begin{table*}[htbp]
    \centering
    \begin{tabular}{c|l}
        \toprule
        Room Types & `office', `kitchen', `bathroom', `apartment', `living room / lounge', `bedroom / hotel' \\
        \midrule
        Object Categories & `chair', `table', `computer', `curtain', `sink', `bed', `bookcase', `sofa', `toilet', `tub' \\
        \bottomrule
    \end{tabular}
    \caption{\textbf{Experiment Settings.} We select 6 room types and 10 object categories for training and validation to minimize distribution shift.}
    \label{tab:experiment_settings}
\end{table*}

\lstset{
    basicstyle=\ttfamily\footnotesize,
    backgroundcolor=\color{gray!9},
    frame=single,
    breaklines=true,
}

\begin{lstlisting}[caption=Prompt of the LLM Backbone, label=lst:1]
<|point_start|><|point_pad|><|point_end|>Detect chair, table, computer, curtain, sink, bed, bookcase, sofa, toilet, tub. The reference code is as followed:
@dataclass
class Wall:
    ax: int
    ay: int
    az: int
    bx: int
    by: int
    bz: int
    height: int
    thickness: int

@dataclass
class Door:
    wall_id: str
    position_x: int
    position_y: int
    position_z: int
    width: int
    height: int

@dataclass
class Window:
    wall_id: str
    position_x: int
    position_y: int
    position_z: int
    width: int
    height: int

@dataclass
class Bbox:
    class: str
    position_x: int
    position_y: int
    position_z: int
    angle_z: int
    scale_x: int
    scale_y: int
    scale_z: int
\end{lstlisting}

\noindent \textbf{Experiment Settings} Some room types in ScanNet and ScanNet++ are not suitable for SpatialLM~\cite{mao2025spatiallm} (SpatialLM lacks relevant prior knowledge). In our experiments, we choose a subset of room types, as well as 10 object categories for training and validation to minimize the distribution shift of data, as shown in Tab.~\ref{tab:experiment_settings}. Following SpatialLM, the prompt we use for the LLM backbone is demonstrated in Lst.~\ref{lst:1}. We replace \texttt{<|point\_pad|>} with the spatial memory tokens for inference.

\noindent \textbf{Baseline Settings} Here we illustrate some implementation details of the baselines. \textbf{1.} In SpatialLM-Merge, for each newly predicted bounding box, we will match it against existing bounding boxes of the same type using the Hungarian algorithm. If the IoU of the matched bounding box is greater than 0.25, the matched bounding box will be updated as the new bounding box. \textbf{2.} In the two ground-truth baselines, we project the depth map to 3D as the ground-truth point cloud of each frame. In addition, for the training of all baselines we use ground-truth point clouds and semantic labels. The difference between lower-bound baselines and ground-truth baselines is whether the ground-truth data is available during inference.
